# Supplementary material for: Nteasee: Understanding Needs in AI for Health in Africa -- A Mixed-Methods Study of Expert and General Population Perspectives
Source: arXiv:2409.12197 source file (2025-05-25)
Supplement: Supplementary file 1 [file interview.pdf]

# Nteasee study expert in-depth interviews

**Interview Script - Experts**

Thank you for agreeing to be here today, I would like to hear your thoughts on artificial intelligence and health equity in Africa. The goal of this interview is to understand the best practices and potential biases to mitigate when deploying AI for health in African countries, as well as explore opportunities where AI could make a positive impact in health. There are no right or wrong answers today. We will not share any information that can be linked to you, so please feel free to share your thoughts openly and be as honest as possible. The information gathered today will be used to write a research paper that will be published in a journal. I will audio record today's discussion. This session should last approximately 1 hour, and you can opt out at anytime. Do you have any questions? (~5 mins)

---

**Section 1**

*I am first going to ask you some questions on health inequities in Africa.(HE)*
(Objective: understand current health inequities and general thoughts on addressing inequities)
(Research question: understand current health inequities and general thoughts on addressing inequities)

1) What do health inequities look like to you in the context of African countries?

*The WHO defines health inequities as "differences in health status or in the distribution of health resources between different population groups, arising from the social conditions in which people are born, grow, live, work and age"*

2) Would you modify this definition in any way?
3) What do you think most impacts health inequities?
    a) Probe: For example, gender, religion, ethnicity
4) What are some approaches you think could be used to help address these inequities?
    a) Probe: Think about something you, your network, companies, or government officials could do
    b) Probe: what can be done by people on the ground

*Now I am going to ask you questions concerning machine learning or Artificial intelligence and health. The Oxford dictionary defines AI as "**the study and***

***development of computer systems that can copy intelligent human behavior*”** *and ML as “***the use and development of computer systems that are able to learn and adapt without following explicit instructions, by using algorithms and statistical models to analyze and draw inferences from patterns in data***.” Depending on who you are, these might mean different things to you or the same thing. For the purposes of this interview, and to appeal to a broader audience I will use the terms AI and machine learning interchangeably.*
(Objective: understand present perceptions around AI and healthcare and opportunities for development)

5) Would you modify the definition in any way in the context of Africa?
6) From your understanding what is the current state of AI in health in the African context? **(MLH)**
7) Do you believe the general population has knowledge of AI or opportunities AI can bring in Healthcare?
    a) Do you believe health workers have knowledge of AI or opportunities AI can bring in Healthcare?
8) How can AI-aided decision-making contribute to improving health outcomes in Africa? **(MLH)**
9) Do you believe there are any barriers to entry to the use of AI in healthcare in Africa?
10) What should be done to ensure that AI research and development is relevant in an African medical context? **(MLH)**
    a) Probe:eg. relevant to cultural use cases, contextually aware of local approaches, optimizing positive health outcomes in Africa
11) Are there opportunities you can think of for AI methods and tools to be applied to address **health inequities** in Africa? **(HE)**
    a) Probe: What are the key areas/sectors of intervention?

*Most African countries were colonized and there are arguments that the effects of colonial history continue to pose a challenge towards African countries. The next few questions ask about your thoughts on colonial history and how that may or may not impact AI.*
(Objective: understand the effects of colonial history on AI)

12) From your perspective, **with respect to colonialism**, is the application of AI to health in African countries and former colonial territories impacted by the history of colonialism? (CGNS)
13) Continuing to think about **the impact of colonialism**, what do you perceive as unique challenges in the application of AI to health faced by African countries and former colonial territories?

   a) Probe: Are there specific challenges you can think of related to colonial history?

14) With respect to **colonialism/colonial history**, do you perceive any social benefits involved in the application of AI to African countries and former colonial spaces?
   a) If yes, what are some of the social benefits you can think of?

15) With respect to **colonialism/colonial history**, do you perceive any social dangers involved in the application of AI to African countries and former colonial spaces?
   a) If yes, what are some of the social dangers you can think of?

*The next set of questions seek to understand your thoughts on fairness and bias considerations in AI for health in Africa and potential sources of AI biases.*
(Objective: Identify gaps in fairness and ML bias for African contexts)

16) Can you describe what comes to mind when you hear
   a) Bias in Artificial Intelligence/Machine learning

*Now bias has several definitions and mean different things to different people, for the purposes of this study–and for the purposes of providing an anchor point particularly for people who may be unfamiliar, we use the definition of bias as "**a phenomenon that occurs when an algorithm produces results that may be harmful due to erroneous assumptions or elements in the Machine Learning or Artificial Intelligence process. In healthcare specifically, this may also be explained as when an algorithm results in different treatment and/or outcomes for different people differently as a result of (1) inequalities in historical and/or current methods in health care access and delivery, (2) data limitations such as unequal representation, errors with measurement, and missing data and (3) differences in access, ability to use or effectiveness across different groups of people (Pfohl et al. 2021)**".*

17) Would you modify the definition in any way in the context of Africa?

18) Given this definition, what do you believe would be sources of algorithmic bias in the African context for AI in healthcare?
   a) Probe: what sources of bias you think can appear at each step of the ML development pipeline. [Show picture of ML pipeline]

19) Do you believe AI is likely to replicate stereotypes and bias about various sub-groups and cultures across Africa, e.g., ethnic identities, religion, countries, gender, etc.?

a) [Follow up to yes] Do you think this poses a serious challenge to effective AI initiatives in Africa, and what can be done to address it? (SV)
b) [Follow up to no] Could you elaborate? (SV)

20) Can you describe what comes to mind when you hear
    a) Fairness in Machine learning/ AI

*Fairness is commonly understood as "**the process of understanding, identifying, correcting and eliminating algorithmic harms/bias from machine learning models.**"*

21) Would you modify the definition in any way in the context of Africa?
22) Are algorithmic fairness considerations relevant to AI application in African countries?
    a) If it is, how should it be thought of?
23) Based on your understanding of AI and of various health needs across Africa, what would a fair AI system in health look like in Africa?

*Now I would like to get your thoughts on methods to design AI solutions for health in Africa*

(Objective: proposal or community-driven solutioning for representative data generation and design and deployment of models)

24) From your perspective how can communities drive the design and deployment of AI systems that affect them?
    a) How can/should communities in Africa be involved in AI initiatives intended for them? (MLF)
25) What is the significance of digital literacy in Africa for optimizing the effectiveness of AI initiatives in the region?
    a) Probe: How can digital literacy needed for AI competency be achieved across Africa?
    b) Probe: How specifically? (MLF)

*Ade-Ibijola & Okonkwo in a [2023 article] write that "...there is a data scarcity in Africa [...] [and] the majority of acquired data does not correctly reflect the African experience, implying that many algorithms may not be appropriately adapted to the features of local populations."*

26) What are your thoughts on this statement?
27) What in your opinion can be done to address the data scarcity issue in Africa?
28) Does it require compromising on important values at stake, e.g., privacy and data sovereignty?

**Section 2**
*In this section I will present you with a thought case modeling real-life AI/ML use cases and ask questions related to it.*
—---------------------------------------------------------------------------------------------------------
**Thought-case #C [All]-**

(MLH) Imagine there is a smartphone application that allows a person to obtain general and preliminary medical advice via text-/speech-communication with a ChatBot trained in medical diagnosis and counseling. This ChatBot is capable not only of receiving information about medical concerns, but can also analyze and diagnose medical conditions from images and patients' descriptions of symptoms. The chatbot is being used by a hospital in Uganda to answer patient's questions.

1. In your opinion, what considerations should be made before deployment of the ChatBot tool?
2. In your opinion, what information should the ChatBot tool present from the outset in order for a user to maximize the value of such a tool?
3. In your opinion, what information would it be necessary/important for the user to give to the ChatBot in order for it to adequately provide medical diagnosis and counseling?
4. In your opinion, what information would it be necessary/important for the ChatBot to be equipped with in order for it to distinguish urgent/emergency medical cases from other sorts of cases?
5. On a scale of 1-10 with 1 being 'not at all' and 10 being 'completely trust', how much would you trust the ChatBot tool for your health?
    a. Follow up: What would need to happen to increase your trust in the chatbot
    b. Follow up: What would need to happen to decrease your trust in the chatbot

**Are there any additional comments or questions you have related to this study that we did not cover during the interview?**

*Thank you so much for your time. We have come to the end of the interview. Please remember to fill out your pre-interview survey if you have not done so already. We will follow up shortly with the interview incentive once the study team receives all of your materials. Thank you again and have a good day/night*

END OF INTERVIEW

---

**Thought-case #A[Clinicians only] -**

(MLH) Imagine you are a clinician using an AI-based software that has been developed in a different country (let's say the USA) and you plan to use the software to assist you in providing diagnosis to your patients. Imagine that the software can take in patient radiology images and previous health records to provide the diagnosis. The software has excellent performance however, (1) it requires historical health records to reach the best performance it can, (2) it was developed using radiology images from a different device than what you use, (3) it has been shown to perform worse for African-Americans.

1. How do you approach using the tool for diagnosing your patients?
2. Which of the following will most impact your decision to use the tool and why?
    - ☐ (1) - it requires historical health records to reach the best performance it can
    - ☐ (2) - it was developed using radiology images from a different device than what you use
    - ☐ (3) - it has been shown to have worse performance for African-Americans
3. Which of the following will least impact your decision to use the tool and why?
    - ☐ (1) - it requires historical health records to reach the best performance it can
    - ☐ (2) - it was developed using radiology images from a different device than what you use
    - ☐ (3) - it has been shown to have worse performance for African-Americans
4. On a scale of 1 to 10 with 1 being no reliability at all, and 10 being highest reliability, how much would you rate your ability to rely on the AI diagnosis model in light of its reported limitations?

5. You now have specific information that your model has a 70% prediction accuracy for a certain ethnic group in your country (let's call this group A) vs. 90% prediction accuracy for the rest of the population. Do your responses above change and why?

**Thought-case #B [All]-**

(CGNS) Imagine you are a researcher and undertake a data collection campaign for skin conditions (e.g., skin lesions, malign moles, allergic reactions such as hives or

rashes, etc.) in one or more Sub-Saharan African countries. This may involve collecting medical images from hospitals and clinics, as well as receiving (credible) photo submissions from individuals suffering from said conditions. The compiled data is to be used in a variety of AI training and testings.

1. What in your opinion would be the top three best practices for collecting data?
2. What do you consider the worst 3 bad practices for collecting data?

**Section 3**

*AI models may perform differently across different groups of people or different locations for a variety of reasons. This section seeks to understand what this looks like in Africa.*

Would any of the following cause an **AI tool for health** to perform differently for people in Africa (you can reference your specific country) and whether it would be worse or better for citizens of your country. (SV) **Respond with better, worse, or same, followed by why**

- ☐ Country of birth
- ☐ Country of residence
- ☐ Colonial history of country of origin
- ☐ National income level (i.e economic performance of country)
- ☐ Race (Black, White, Asian, Mixed race, etc)
- ☐ Ethnic group
- ☐ Skin tone
- ☐ Religion
- ☐ Language
- ☐ Gender (male, female, transgender, non-binary, etc)
- ☐ Sexual orientation (attracted to people of opposite gender, attracted to people of the same gender as self, attracted to people of any gender, not attracted to anyone, etc)
- ☐ Literacy and education level
- ☐ Rural or urban location of residence
- ☐ Family income level
- ☐ A disability
- ☐ Any pre-existing health conditions (eg. high blood pressure, diabetes, asthma, or others)
- ☐ Genetics

- [ ] Phenotype (i.e, body look, shape, weight, height, etc compared to others)

*You have come to the end of the interview. Do you have anything to add that I have not yet asked? Thank you so much for your time.*

—-----------------------------------------------------------------------------------------------------------

—-----------------------------------------------------------------------------------------------------------
